# Supplementary material for: Electro-Chemo-Mechanical Model for Polymer Electrolytes
Source: arXiv:2306.16157 ancillary file (2024-03-05)
Supplement: Supplementary file 1 [file SuppInfo.pdf]

# Supporting Information: Electro-Chemo-Mechanical Model for Polymer Electrolytes


Daniel O. Möhrle,[1,2] Katharina Becker-Steinberger,[1,2] Max Schammer,[1,2] Birger Horstmann,[1,2,3,*] and Arnulf Latz[1,2,3,†]

[1] *German Aerospace Center, Wilhelm-Runge-Straße 10, 89081 Ulm, Germany*
[2] *Helmholtz Institute Ulm, Helmholtzstraße 11, 89081 Ulm, Germany*
[3] *Universität Ulm, Albert-Einstein-Allee 47, 89081 Ulm, Germany*


**CONTENTS**


S1. Transport Theory 1
  A. Entropy flux frame transformation 1
  B. Polymer velocity and incompressibility 3
  C. Consistent chemo-mechanical coupling 4
  D. Evaluation of driving forces 5
  E. Reduction of the polymer transport model 6
  F. Volume-frame 7

S2. Simulation 8
  A. Parameters 8
    1. PEO/LiTFSI 8
    2. SIC/EC 9
  B. Numerical Methods 9
  C. Thermodynamic transport contributions 9

S3. Steady state and polymer deformation 11

References 14


## S1. TRANSPORT THEORY

### A. Entropy flux frame transformation

In this section we give a detailed derivation of the entropy production rate $R_\text{s}$, and expand it with respect to the polymer frame using flux-force pairs (see section II A).
First, we calculate the total differential of the Helmholtz free energy density $\rho\dot{\varphi}_\text{H}$ (see also eq. (11)),

$$\rho\dot{\varphi}_\text{H} = -\rho s\cdot\dot{T} - \sum_{\alpha=1}^{N} \upmu_\alpha \cdot \text{div}\left(\boldsymbol{N}_\alpha\right) + \boldsymbol{\mathcal{E}}\cdot\dot{\boldsymbol{D}} + \boldsymbol{\mathcal{H}}\cdot\dot{\boldsymbol{B}} + \boldsymbol{\sigma} : \left[\text{grad}\left(\boldsymbol{d}_\text{p}\right) - \left(\boldsymbol{d}_\text{p}\cdot\text{grad}\left(\boldsymbol{F}\right)\right)\cdot\boldsymbol{F}^{-1}\right] + \left(\boldsymbol{\sigma} + \left[\rho\varphi_\text{H} - \sum_{\alpha=1}^{N}\upmu_\alpha c_\alpha\right]\mathbb{1}\right) : \text{grad}\left(\boldsymbol{v}\right). \quad \text{(S1)}$$

Above, we have used eqs. (1), (2) and (5) to express the material derivative of the deformation gradient tensor $\boldsymbol{F}$ via the velocity difference between the polymer velocity and the center-of-mass velocity $\boldsymbol{d}_\text{p} = \boldsymbol{v}_\text{p} - \boldsymbol{v}$ (*cf.* eq. (5)). From


* birger.horstmann@dlr.de
† arnulf.latz@dlr.de

eq. (S1) and using balance of internal energy in addition to the Legendre-transformation $\rho\varphi_{\mathrm{H}} = \rho u - T\rho s$, it follows the balance equation for the entropy density,

$$\begin{aligned} T\rho\dot{s} =& \rho\dot{u} - \rho\dot{\varphi}_{\mathrm{H}} - \rho s\dot{T} \\ =& \boldsymbol{v}\cdot\left(\rho\dot{\boldsymbol{g}} - \rho\dot{\boldsymbol{v}} - (\boldsymbol{D}\dot{\times}\boldsymbol{B})\right) + \rho h \\ &+ \left(\boldsymbol{\tau} - \boldsymbol{\sigma} - \boldsymbol{\mathcal{E}}\otimes\boldsymbol{D} - \boldsymbol{\mathcal{H}}\otimes\boldsymbol{B} - \left(\rho\varphi_{\mathrm{H}} - \sum_{\alpha=1}^{\mathrm{N}}\mu_\alpha c_\alpha - \boldsymbol{\mathcal{E}}\cdot\boldsymbol{D} - \boldsymbol{\mathcal{H}}\cdot\boldsymbol{B}\right)\mathbb{1}\right) : \mathrm{grad}\,(\boldsymbol{v}) \\ &- \mathrm{div}\left(\boldsymbol{q} - \sum_{\alpha=1}^{\mathrm{N}}\mu_\alpha\boldsymbol{N}_\alpha + \boldsymbol{d}_{\mathrm{p}}\cdot\boldsymbol{\sigma}\right) + \boldsymbol{\mathcal{E}}\cdot\boldsymbol{\mathcal{J}} \\ &- \sum_{\alpha=1}^{\mathrm{N}}\boldsymbol{N}_\alpha\cdot\mathrm{grad}\,(\mu_\alpha) + \boldsymbol{d}_{\mathrm{p}}\cdot\left[\mathrm{div}\,(\boldsymbol{\sigma}) + \left(\mathrm{grad}\,(\boldsymbol{F})\cdot\boldsymbol{F}^{-1}\right):\boldsymbol{\sigma}\right]. \end{aligned} \tag{S2}$$

Note that the entropy flux density $\boldsymbol{j}_{\mathrm{s}}$ is yet not defined. However, in addition to eq. (S2), there exists the Clausius-Duhem inequality $T\rho\dot{s} = R_{\mathrm{s}} + \rho h - T\mathrm{div}(\boldsymbol{j}_{\mathrm{s}})$. This closes the form for the entropy flux density, $\boldsymbol{j}_{\mathrm{s}} = (\boldsymbol{q} - \sum_{\alpha=1}^{N}\mu_\alpha\boldsymbol{N}_\alpha + \boldsymbol{d}_{\mathrm{p}}\cdot\boldsymbol{\sigma})/T$, and determines the entropy production rate,

$$\begin{aligned} R_{\mathrm{s}} =& \boldsymbol{v}\cdot\left(\rho\dot{\boldsymbol{g}} - \rho\dot{\boldsymbol{v}} - (\boldsymbol{D}\dot{\times}\boldsymbol{B})\right) \\ &+ \left(\boldsymbol{\tau} - \boldsymbol{\sigma} - \boldsymbol{\mathcal{E}}\otimes\boldsymbol{D} - \boldsymbol{\mathcal{H}}\otimes\boldsymbol{B} - \left(\rho\varphi_{\mathrm{H}} - \sum_{\alpha=1}^{\mathrm{N}}\mu_\alpha c_\alpha - \boldsymbol{\mathcal{E}}\cdot\boldsymbol{D} - \boldsymbol{\mathcal{H}}\cdot\boldsymbol{B}\right)\mathbb{1}\right) : \mathrm{grad}\,(\boldsymbol{v}) \\ &+ \boldsymbol{\mathcal{E}}\cdot\boldsymbol{\mathcal{J}} - \boldsymbol{j}_{\mathrm{s}}\cdot\mathrm{grad}\,(T) - \sum_{\alpha=1}^{\mathrm{N}}\boldsymbol{N}_\alpha\cdot\mathrm{grad}\,(\mu_\alpha) + \boldsymbol{d}_{\mathrm{p}}\cdot\left[\mathrm{div}\,(\boldsymbol{\sigma}) + \left(\mathrm{grad}\,(\boldsymbol{F})\cdot\boldsymbol{F}^{-1}\right):\boldsymbol{\sigma}\right]. \end{aligned} \tag{S3}$$

Next, we derive the constitutive equations of our polymer theory. Here, we follow the rationale outlined by Kovetz in Ref. 1. The initial choice of the set of material variables $\mathbb{V}_0 = \{T, \boldsymbol{F}, c_\alpha, \boldsymbol{D}, \boldsymbol{B}\}$ determines the free energy and, by extension through the constitutive equations eqs. (12) to (16), the set of quantities $\{s, \boldsymbol{\sigma}, \mu_\alpha, \boldsymbol{\mathcal{E}}, \boldsymbol{\mathcal{H}}\}$. The initial center-of-mass velocity $\boldsymbol{v}$ (and there fore also $\mathrm{grad}\,(\boldsymbol{v})$) can be chosen independently of $\mathbb{V}_0$. The second law of thermodynamics dictates the entropy production rate eq. (S3) to be non-negative. To prevent a negative entropy production due to the first or second term in eq. (S3), we choose the up until now undetermined generalized stress tensor $\boldsymbol{\tau}$ and the change of the total momentum density $\rho\dot{\boldsymbol{g}}$ in such a way that the factors of $\boldsymbol{v}$ and $\mathrm{grad}\,(\boldsymbol{v})$ in eq. (S3) vanish. This leads to the additional constitutive equations for the momentum density $\rho\dot{\boldsymbol{g}}$:

$$\rho\dot{\boldsymbol{g}} = \rho\dot{\boldsymbol{v}} + \frac{\mathrm{d}}{\mathrm{d}t}\left(\boldsymbol{D}\times\boldsymbol{B}\right), \tag{S4}$$

and the generalized stress tensor,

$$\boldsymbol{\tau} = \boldsymbol{\sigma} + \boldsymbol{\mathcal{E}}\otimes\boldsymbol{D} + \boldsymbol{\mathcal{H}}\otimes\boldsymbol{B} + \left(\rho\varphi_{\mathrm{H}} - \sum_{\alpha=1}^{\mathrm{N}}\mu_\alpha c_\alpha - \boldsymbol{\mathcal{E}}\cdot\boldsymbol{D} - \boldsymbol{\mathcal{H}}\cdot\boldsymbol{B}\right)\mathbb{1}. \tag{S5}$$

With these constitutive equations, eq. (S3) reduces to

$$R_{\mathrm{s}} = \boldsymbol{\mathcal{E}}\cdot\boldsymbol{\mathcal{J}} - \boldsymbol{j}_{\mathrm{s}}\cdot\mathrm{grad}\,(T) - \sum_{\alpha=1}^{\mathrm{N}}\boldsymbol{N}_\alpha\cdot\mathrm{grad}\,(\mu_\alpha) + \boldsymbol{d}_{\mathrm{p}}\cdot\left[\mathrm{div}\,(\boldsymbol{\sigma}) + \left(\mathrm{grad}\,(\boldsymbol{F})\cdot\boldsymbol{F}^{-1}\right):\boldsymbol{\sigma}\right]. \tag{S6}$$

We simplify this expression using $\boldsymbol{\mathcal{J}} = \sum_{\alpha=1}^{\mathrm{N}} F z_\alpha \boldsymbol{N}_\alpha$, and expressing the electric field via the electric potential $\boldsymbol{\mathcal{E}} = -\mathrm{grad}\,(\phi)$, such that

$$R_{\mathrm{s}} = -\sum_{\alpha=1}^{N}\boldsymbol{N}_\alpha\cdot\boldsymbol{\mathcal{F}}_\alpha^{\mathrm{el}} - \boldsymbol{j}_{\mathrm{s}}\cdot\boldsymbol{\mathcal{F}}_{\mathrm{T}} - \boldsymbol{N}_{\mathrm{p}}\cdot\boldsymbol{\mathcal{F}}_{\mathrm{mech}}, \tag{S7}$$

where we introduce N+2 mechanical, electro-chemical and thermal forces

$$\boldsymbol{\mathcal{F}}_\alpha^{\mathrm{el}} = \mathrm{grad}(\mu_\alpha^{\mathrm{el}}), \quad \boldsymbol{\mathcal{F}}_{\mathrm{T}} = \mathrm{grad}(T), \quad \text{and} \quad \boldsymbol{\mathcal{F}}_{\mathrm{mech}} = -\frac{1}{c_{\mathrm{p}}}\left[\mathrm{div}(\boldsymbol{\sigma}) + \left(\mathrm{grad}(\boldsymbol{F})\cdot\boldsymbol{F}^{-1}\right):\boldsymbol{\sigma}\right]. \tag{S8}$$

Here, $\mu_\alpha^{\text{el}} = \mu_\alpha + Fz_\alpha\Phi$ is the electrochemical potential.

Next, we ensure non-negativity of eq. (S7) and choose the closure relation for the yet undefined fluxes. For this purpose, we choose an linear Onsager approach for the flux-force relation. However, before we do so, we transform the forces and fluxes to the reference frame defined by the internal species velocity of the polymer,[2]

$$\boldsymbol{N}_\alpha^{\text{p}}|_{\alpha\neq\text{p}} = c_\alpha\left(\boldsymbol{v}_\alpha - \boldsymbol{v}_\text{p}\right) = c_\alpha\left(\boldsymbol{v}_\alpha - \boldsymbol{v}\right) + c_\alpha\left(\boldsymbol{v} - \boldsymbol{v}_\text{p}\right) = \boldsymbol{N}_\alpha - \frac{c_\alpha}{c_\text{p}}\boldsymbol{N}_\text{p} = \boldsymbol{N}_\alpha + \sum_{\beta=2}^{\text{N}} \frac{c_\alpha}{c_\text{p}}\frac{M_\beta}{M_\text{p}}\boldsymbol{N}_\beta. \tag{S9}$$

In the last step, we made use of the mass-based flux constraint $\sum_{\alpha=1}^{\text{N}} M_\alpha \boldsymbol{N}_\alpha = 0$. In matrix form, this reads

$$\boldsymbol{N}_\alpha^{\text{p}} = \sum_{\beta=2}^{\text{N}} A_{\alpha\beta}^{\text{pM}} \cdot \boldsymbol{N}_\beta \quad \text{and} \quad \boldsymbol{N}_\alpha = \sum_{\beta=2}^{\text{N}} A_{\alpha\beta}^{\text{Mp}} \cdot \boldsymbol{N}_\beta^{\text{p}}, \tag{S10}$$

where

$$A_{\alpha\beta}^{\text{pM}} = \left(\delta_{\alpha\beta} + \frac{c_\alpha M_\beta}{c_\text{p} M_\text{p}}\right) \quad \text{and} \quad A_{\alpha\beta}^{\text{Mp}} = \left(A_{\alpha\beta}^{\text{pM}}\right)^{-1} = \left(\delta_{\alpha\beta} - \frac{c_\alpha M_\beta}{\rho}\right). \tag{S11}$$

In a similar way, we obtain the entropy flux density in the polymer frame,[3]

$$\boldsymbol{j}_\text{s}^{\text{p}} = \rho s\left(\boldsymbol{v}_\text{s} - \boldsymbol{v}_\text{p}\right) = \rho s\left(\boldsymbol{v}_\text{s} - \boldsymbol{v}\right) + \rho s\left(\boldsymbol{v} - \boldsymbol{v}_\text{p}\right) = \boldsymbol{j}_\text{s} - \frac{\rho s}{c_\text{p}}\boldsymbol{N}_\text{p} = \boldsymbol{j}_\text{s} + \sum_{\alpha=2}^{\text{N}} \frac{\rho s M_\alpha}{c_\text{p} M_\text{p}}\boldsymbol{N}_\alpha = \boldsymbol{j}_\text{s} + \sum_{\alpha,\beta=2}^{\text{N}} \frac{\rho s M_\alpha}{c_\text{p} M_\text{p}} A_{\alpha\beta}^{-1}\boldsymbol{N}_\beta^{\text{p}}. \tag{S12}$$

Finally, the entropy production rate eq. (S7) expressed with respect to the polymer-frame fluxes reads

$$\begin{aligned} R_\text{s} &= -\sum_{\alpha=1}^{N} \boldsymbol{N}_\alpha \cdot \boldsymbol{\mathcal{F}}_\alpha^{\text{el}} - \boldsymbol{j}_\text{s} \cdot \boldsymbol{\mathcal{F}}_\text{T} - \boldsymbol{N}_\text{p} \cdot \boldsymbol{\mathcal{F}}_\text{mech} \\ &= -\sum_{\alpha=2}^{N} \boldsymbol{N}_\alpha \cdot \left(\boldsymbol{\mathcal{F}}_\alpha^{\text{el}} - \frac{M_\alpha}{M_\text{p}}\left(\boldsymbol{\mathcal{F}}_\text{p}^{\text{el}} + \boldsymbol{\mathcal{F}}_\text{mech}\right)\right) - \boldsymbol{j}_\text{s} \cdot \boldsymbol{\mathcal{F}}_\text{T} \\ &= -\sum_{\alpha,\beta=2}^{N} A_{\alpha\beta}^{-1} \cdot \boldsymbol{N}_\beta^{\text{p}} \cdot \left(\boldsymbol{\mathcal{F}}_\alpha^{\text{el}} - \frac{M_\alpha}{M_\text{p}}\left(\boldsymbol{\mathcal{F}}_\text{p}^{\text{el}} + \boldsymbol{\mathcal{F}}_\text{mech}\right)\right) - \left(\boldsymbol{j}_\text{s}^{\text{p}} - \sum_{\alpha,\beta=2}^{\text{N}} \frac{\rho s M_\alpha}{c_\text{p} M_\text{p}} A_{\alpha\beta}^{-1}\boldsymbol{N}_\beta^{\text{p}}\right) \cdot \boldsymbol{\mathcal{F}}_\text{T}^{\text{p}} \\ &= -\sum_{\alpha=2}^{\text{N}} \boldsymbol{N}_\beta^{\text{p}} \cdot \boldsymbol{\mathcal{F}}_\alpha^{\text{el,p}} - \boldsymbol{j}_\text{s}^{\text{p}} \cdot \boldsymbol{\mathcal{F}}_\text{T}^{\text{p}}, \end{aligned} \tag{S13}$$

with the electro-chemo-mechanical and thermal driving forces in the polymer reference frame

$$\boldsymbol{\mathcal{F}}_\beta^{\text{el,p}} = \sum_{\alpha=2}^{\text{N}} \left(\boldsymbol{\mathcal{F}}_\alpha^{\text{el}} - \frac{M_\alpha}{M_\text{p}}\left[\boldsymbol{\mathcal{F}}_\text{mech} + \frac{\rho s}{c_\text{p}}\boldsymbol{\mathcal{F}}_\text{T} + \boldsymbol{\mathcal{F}}_\text{p}^{\text{el}}\right]\right) A_{\alpha\beta}^{-1}, \tag{S14}$$

and

$$\boldsymbol{\mathcal{F}}_\text{T}^{\text{p}} = \text{grad}\left(T\right) = \boldsymbol{\mathcal{F}}_\text{T}. \tag{S15}$$

Note that the thermal driving forces are identical in the different reference frames.

### B. Polymer velocity and incompressibility

In this section we briefly discuss microscopic incompressibility, state the equation for the polymer convection velocity, and identify the number of independent species concentrations.

As was presented in great detail by Schammer et.al. (see Ref. 4), the partial molar volumes are completely determined by the stress tensor / pressure forces in our formalism. In the incompressible limit, where the partial

molar volumes do not depend on the pressure, the partial molar volumes are identical to the reference quantities introduced in the main text $\nu_\alpha = \nu_\alpha^0$ . Furthermore, in the incompressible limit, the equation for the polymer convection velocity reads,[2,4]

$$\operatorname{div}(\boldsymbol{v}_\mathrm{p}) = -\sum_{\alpha=2}^{\mathrm{N}} \nu_\alpha \operatorname{div}(\boldsymbol{N}_\alpha^\mathrm{p}) \,. \tag{S16}$$

Finally, we evaluate the following three relations between the species concentrations and the volume deformation and reduce the set of independent variables,

$$\det(\boldsymbol{F}) = J = \frac{1}{\nu_\mathrm{p} c_\mathrm{p}} \ , \ \varrho^\mathrm{F} = \sum_{\alpha=1}^{\mathrm{N}} F z_\alpha c_\alpha \ , \text{ and } \ 1 = \sum_{\alpha=1}^{\mathrm{N}} \nu_\alpha c_\alpha \tag{S17}$$

We use these three constraints and eliminate the three species $c_\mathrm{p}, c_2, c_3$ from the set of independent variables of state, such that $\mathbb{V}_1 = \{T, \boldsymbol{F}, \varrho^\mathrm{F}, c_4, ..., c_\mathrm{N}, \boldsymbol{D}, \boldsymbol{B}\}$, where

$$c_1 = c_\mathrm{p} = \frac{1}{\nu_\mathrm{p} J} = \frac{1}{\nu_\mathrm{p} \det(\boldsymbol{F})}, \tag{S18}$$

$$c_2 = \left[ z_3 - \left( z_3 - \frac{\nu_3}{\nu_\mathrm{p}} z_\mathrm{p} \right) \frac{1}{J} - \nu_3 \cdot \frac{\varrho^\mathrm{F}}{F} + \sum_{\alpha=4}^{\mathrm{N}} (\nu_3 z_\alpha - \nu_\alpha z_3)\, c_\alpha \right] / \left[ \nu_2 z_3 - \nu_3 z_2 \right], \tag{S19}$$

$$c_3 = \left[ z_2 - \left( z_2 - \frac{\nu_2}{\nu_\mathrm{p}} z_\mathrm{p} \right) \frac{1}{J} - \nu_2 \cdot \frac{\varrho^\mathrm{F}}{F} + \sum_{\alpha=4}^{\mathrm{N}} (\nu_2 z_\alpha - \nu_\alpha z_2)\, c_\alpha \right] / \left[ \nu_3 z_2 - \nu_2 z_3 \right]. \tag{S20}$$

### C. Consistent chemo-mechanical coupling

In this section, we calculate the chemical potentials, stresses and pressure forces as determined from our model free energy density, see eq. (30), by the constitutive eqs. (13) and (14). Furthermore, we discuss the kinematical limit which closes our constitutive modeling for the fully mechanically coupled forces.[4]

The volumetric contribution to our model for the Helmholtz free energy density, $\mathcal{K}/2\cdot(1 - \sum_{\alpha=1}^{\mathrm{N}} \nu_\alpha^0 c_\alpha)^2$, leads to pressure forces $\mathcal{P} = -\mathcal{K} \cdot (1 - \sum_{\alpha=1}^{\mathrm{N}} \nu_\alpha c_\alpha)$ appearing in the total stress tensor $\boldsymbol{\tau}$. However, using these pressure-like forces eq. (14):

$$\mu_\alpha = \mu_\alpha^0 + \nu_\alpha^0 \mathcal{P} + RT \Big[ 1 + \log(\nu_\alpha^0 c_\alpha) + \nu_\alpha^0 \sum_{\substack{\beta=1 \\ \beta\neq\alpha}}^{\mathrm{N}} \xi_{\alpha\beta} \nu_\beta^0 c_\beta \Big]. \tag{S21}$$

Next, we split the total stress tensor into it's isotropic trace-part given by pressure forces $p$, and it's anisotropic deviatoric part $\boldsymbol{\tau}^\mathrm{dev}$,

$$\boldsymbol{\tau} = -p\mathbb{1} + \boldsymbol{\tau}^\mathrm{dev}, \quad \text{where} \quad p = -\frac{1}{3}\operatorname{tr}(\boldsymbol{\tau}), \quad \text{and} \quad \boldsymbol{\tau}^\mathrm{dev} = \boldsymbol{\tau} + p\mathbb{1}. \tag{S22}$$

For our choice of the Helmholtz free energy (see eq. (30)), the detailed expressions are

$$p = \mathcal{P} - \frac{1}{2}\frac{K_\mathrm{p}}{J}\left(J^2 - 1\right) + \frac{1}{6}\left(\boldsymbol{\mathcal{E}}\cdot\boldsymbol{D} + \boldsymbol{\mathcal{H}}\cdot\boldsymbol{B}\right) + RT\Big[ c + \frac{1}{2} \sum_{\substack{\alpha,\beta=1 \\ \alpha\neq\beta}}^{\mathrm{N}} \xi_{\alpha\beta} \nu_\alpha^0 c_\alpha \nu_\beta^0 c_\beta \Big] \tag{S23}$$

and

$$\boldsymbol{\tau}^\mathrm{dev} = \frac{G_\mathrm{p}}{J^{5/3}} \left( \boldsymbol{F}\cdot\boldsymbol{F}^\mathrm{T} - \frac{\operatorname{tr}\left(\boldsymbol{F}^\mathrm{T}\cdot\boldsymbol{F}\right)}{3}\mathbb{1} \right) + \boldsymbol{\mathcal{E}}\otimes\boldsymbol{D} + \boldsymbol{\mathcal{H}}\otimes\boldsymbol{B} - \frac{1}{3}\left(\boldsymbol{\mathcal{E}}\cdot\boldsymbol{D} + \boldsymbol{\mathcal{H}}\cdot\boldsymbol{B}\right)\mathbb{1} \tag{S24}$$

Replacing the pressure-like forces $\mathcal{P}$ in the chemical potential yields

$$\mu_\alpha = \mu_\alpha^0 + \nu_\alpha^0 p + \frac{1}{2}\nu_\alpha \frac{K_\mathrm{p}}{J}\left(J^2-1\right) - \frac{1}{6}\nu_\alpha\left(\boldsymbol{\mathcal{E}}\cdot\boldsymbol{D} + \boldsymbol{\mathcal{H}}\cdot\boldsymbol{B}\right)$$
$$+ RT\left[\log(\nu_\alpha^0 c_\alpha) + \sum_{\beta=1}^{\mathrm{N}}\left(\nu_\beta^0 - \nu_\alpha^0\right)c_\beta + \frac{1}{2}\sum_{\substack{\beta,\gamma=1\\ \beta\neq\gamma}}^{\mathrm{N}} \xi_{\beta\gamma}\nu_\beta^0\nu_\gamma^0\left(\delta_{\alpha\beta}c_\gamma + \delta_{\alpha\gamma}c_\beta - \nu_\alpha^0 c_\beta c_\gamma\right)\right]. \quad \text{(S25)}$$

Next, we assume that $\mathrm{div}\left(\boldsymbol{\tau}\right) = 0$,[4] such that

$$\begin{aligned}
\mathrm{grad}\left(p\right) =& \mathrm{div}\left(\boldsymbol{\tau}^{\mathrm{dev}}\right)\\
=& \mathrm{div}\left(\frac{G_\mathrm{p}}{J^{5/3}}\boldsymbol{F}\cdot\boldsymbol{F}^\mathrm{T} + \boldsymbol{\mathcal{E}}\otimes\boldsymbol{B} + \boldsymbol{\mathcal{H}}\otimes\boldsymbol{B}\right) - \frac{1}{3}\mathrm{grad}\left(\frac{G_\mathrm{p}}{J^{5/3}}\mathrm{tr}\left(\boldsymbol{F}^\mathrm{T}\cdot\boldsymbol{F}\right) + \boldsymbol{\mathcal{E}}\cdot\boldsymbol{D} + \boldsymbol{\mathcal{H}}\cdot\boldsymbol{B}\right)\\
=& \mathrm{div}\left(\frac{G_\mathrm{p}}{J^{5/3}}\boldsymbol{F}\cdot\boldsymbol{F}^\mathrm{T}\right) - \frac{1}{3}\mathrm{grad}\left(\frac{G_\mathrm{p}}{J^{5/3}}\mathrm{tr}\left(\boldsymbol{F}^\mathrm{T}\cdot\boldsymbol{F}\right)\right) - \left(\varrho^\mathrm{F} + \frac{1}{3}\boldsymbol{D}\cdot\boldsymbol{\nabla}\right)\mathrm{grad}\left(\phi\right).
\end{aligned} \quad \text{(S26)}$$

In the last step, we used $\boldsymbol{\mathcal{H}} = \boldsymbol{B} = 0$ and $\boldsymbol{D} = \epsilon_0\epsilon_\mathrm{r}\boldsymbol{\mathcal{E}}$, with the constant isotropic relative permittivity $\epsilon_\mathrm{r}$. The gradient of the chemical potential appearing in the electrochemical driving forces reads

$$\mathrm{grad}\left(\mu\right)_\alpha = \mathrm{div}\left(\nu_\alpha\frac{G_\mathrm{p}}{J^{5/3}}\boldsymbol{F}\cdot\boldsymbol{F}^\mathrm{T}\right) - \mathrm{grad}\left(\frac{1}{3}\nu_\alpha\frac{G_\mathrm{p}}{J^{5/3}}\mathrm{tr}\left(\boldsymbol{F}^\mathrm{T}\cdot\boldsymbol{F}\right)\right) - \nu_\alpha\varrho^\mathrm{F}\mathrm{grad}\left(\phi\right)$$
$$+ \mathrm{grad}\left(RT\left[\log(\nu_\alpha^0 c_\alpha) + \sum_{\beta=1}^{\mathrm{N}}\left(\nu_\beta^0 - \nu_\alpha^0\right)c_\beta + \frac{1}{2}\sum_{\substack{\beta,\gamma=1\\ \beta\neq\gamma}}^{\mathrm{N}} \xi_{\beta\gamma}\nu_\beta^0\nu_\gamma^0\left(\delta_{\alpha\beta}c_\gamma + \delta_{\alpha\gamma}c_\beta - \nu_\alpha^0 c_\beta c_\gamma\right)\right]\right), \quad \text{(S27)}$$

which couples mechanical forces are and the chemical potentials.

## D. Evaluation of driving forces

The fluxes derived thermodynamically consistent from the entropy inequality appear in the system of equations of motion eqs. (37) to (41). To evaluate the gradients of the chemical potentials $\mu_\alpha$ and the polymer stress tensor $\boldsymbol{\sigma}$, we expand them formally in the variables of state $\mathbb{v}_A \in \mathbb{V}_1$ (eqn. eq. (36)) using the chain-rule for derivatives

$$\mathrm{grad}(\mu_\alpha) = \sum_{\mathbb{v}_A\in\mathbb{V}_1}\left.\frac{\partial\mu_\alpha}{\partial\mathbb{v}_A}\right|_{\mathbb{V}_1}\cdot\mathrm{grad}(\mathbb{v}_A), \quad \text{(S28)}$$

$$\left[\mathrm{div}(\boldsymbol{\sigma})\right]_{ijk} = \sum_{l,m}\frac{\partial\sigma_{ij}}{\partial F_{lm}}\cdot\frac{\partial}{\partial x_k}F_{lm} \quad \text{(S29)}$$

We divide both investigated polymer electrolytes into three species and assume charge neutrality $\varrho^\mathrm{F} = 0$, so the set of material variables of state reduces to $\mathbb{V}_1 = \{\boldsymbol{F}, \Phi\}$. The partial derivatives of the chemical potentials are given by

$$\left.\frac{\partial\mu_\alpha}{\partial\phi}\right|_{\mathbb{V}_1} = 0, \quad \text{(S30)}$$

and

$$\left(\left.\frac{\partial\mu_\alpha}{\partial F_{kl}}\right|_{\mathbb{V}_1}\right)_{ij} = RT\left[\frac{1}{c_\alpha}\frac{\partial c_\alpha}{\partial J} + \sum_{\beta=1}^{\mathrm{N}}\left(\nu_\beta^0 - \nu_\alpha^0\right)\frac{\partial c_\beta}{\partial J} + \sum_{\substack{\beta,\gamma=1\\ \beta\neq\gamma}}^{\mathrm{N}}\frac{\xi_{\beta\gamma}\nu_\beta^0\nu_\gamma^0}{2}\left(\left(\delta_{\alpha\gamma} - \nu_\alpha^0 c_\gamma\right)\frac{\partial c_\beta}{\partial J} + \left(\delta_{\alpha\beta} - \nu_\alpha^0 c_\beta\right)\frac{\partial c_\gamma}{\partial J}\right)\right] J F_{kl}^{-\mathrm{T}}\delta_{ij}$$
$$+ \nu_\alpha\frac{G_\mathrm{p}}{J^{5/3}}\left[-\frac{5}{3}\left(F_{im}F_{mj}^\mathrm{T} - \frac{1}{3}\mathrm{tr}\left(\boldsymbol{F}^\mathrm{T}\cdot\boldsymbol{F}\right)\delta_{ij}\right)F_{kl}^{-\mathrm{T}} + F_{jl}\delta_{ki} + F_{il}\delta_{kj} - \frac{2}{3}F_{kl}\delta_{ij}\right]. \quad \text{(S31)}$$

We use Einstein notation, in which multiple occurring indexes are summed over, with the components $F_{kl}$ of the deformation gradient tensor $\boldsymbol{F}$ and the derivatives of the concentrations with respect to the volume ratio

$$\frac{\partial c_1}{\partial J} = \frac{\partial c_\mathrm{p}}{\partial J} = -\frac{1}{\nu_\mathrm{p}J^2}, \quad \text{and} \quad \frac{\partial c_2}{\partial J} = \frac{\nu_\mathrm{p}z_3 - \nu_3 z_\mathrm{p}}{\nu_2 z_3 - \nu_3 z_2}\cdot\frac{1}{\nu_\mathrm{p}J^2}, \quad \text{and} \quad \frac{\partial c_3}{\partial J} = \frac{\nu_\mathrm{p}z_2 - \nu_2 z_\mathrm{p}}{\nu_3 z_2 - \nu_2 z_3}\cdot\frac{1}{\nu_\mathrm{p}J^2}. \quad \text{(S32)}$$

Using Einstein notation, the total gradient of the chemical potentials is given by

$$\frac{\partial \mu_\alpha}{\partial x_i} = \left( \frac{\partial \mu_\alpha}{\partial F_{kl}}\bigg|_{\mathbb{V}_1} \right)_{ij} \cdot \frac{\partial F_{kl}}{\partial x_j}. \tag{S33}$$

The polymer stress tensor $\boldsymbol{\sigma}$ is obtained by evaluating the corresponding constitutive equation eq. (13)

$$\boldsymbol{\sigma} = G_\mathrm{p} \left( -\frac{5}{6} \mathrm{tr} \left( J^{-\frac{5}{3}} \boldsymbol{F}^\mathrm{T} \cdot \boldsymbol{F} \right) + \frac{3}{2} J^{-1} \right) \mathbb{1} + G_\mathrm{p} J^{-\frac{5}{3}} \boldsymbol{F} \cdot \boldsymbol{F}^\mathrm{T} + \frac{1}{4} K_\mathrm{p} \left( J - J^{-1} + 2J^{-1} \ln(J) \right) \mathbb{1}. \tag{S34}$$

The derivative with respect to $\boldsymbol{F}$ is given by

$$\begin{aligned} \frac{\partial \sigma_{ij}}{\partial F_{mn}} = \frac{1}{J} \Bigg\{ G_\mathrm{p} \Bigg[ \left( \frac{25}{18} \mathrm{tr} \left( J^{-2/3} \boldsymbol{F}^\mathrm{T} \cdot \boldsymbol{F} \right) + \frac{3}{2} \right) \delta_{ij} F^{-\mathrm{T}}_{mn} - \frac{5}{3} J^{-2/3} \left( \delta_{ij} F_{mn} + F_{ik} F^\mathrm{T}_{kj} F^{-\mathrm{T}}_{mn} \right) \\ + J^{-2/3} \left( F^\mathrm{T}_{nj} \delta_{mi} + F_{in} \delta_{mj} \right) \Bigg] + \frac{1}{4} K_\mathrm{p} \left( J^2 + 3 - 2\ln(J) \right) \delta_{ij} F^{-\mathrm{T}}_{mn} \Bigg\}. \end{aligned} \tag{S35}$$

## E. Reduction of the polymer transport model

We validate our transport model and compare it with results discussed by Steinrück and co-workes, see Ref. 5. In this publication, Steinrück et al. discuss the "baseline" polymeric electrolyte given by polyethylene glycol with LiTFSI. Using transport parameters from Pesko et al.[6], the experimental results were compared with results from simulations using concentrated solution theory (CST)[7].

We adapt to their parameterization and transfer to the CST transport parameters assuming that the polymer species dominates the volume-ratio and mass-ratio of the electrolyte species, $\nu_\mathrm{p} c_\mathrm{p} = \frac{1}{J} \approx 1$ and $J \approx 1$. Furthermore, we assume that the partial molar volumes of non-polymer species $\alpha \neq \mathrm{p}$ are much smaller than the polymer partial molar volume, $\nu_\alpha \ll \nu_\mathrm{p}$, which implies that $1 \approx \nu_\mathrm{p} c_\mathrm{p}$ and that $\nu_\alpha c_\alpha \approx 0$ for all species $\alpha \neq \mathrm{p}$. This implies that (see eq. (S25))

$$\mu_\alpha = \mu^0_\alpha + \nu^0_\alpha p - \frac{1}{6} \left( \boldsymbol{\mathcal{E}} \cdot \boldsymbol{D} + \boldsymbol{\mathcal{H}} \cdot \boldsymbol{B} \right) + RT \left[ \log \left( \nu^0_\alpha c_\alpha \right) + \left( 1 - \delta_{\alpha \mathrm{p}} \right) \cdot \left( 1 + \xi_{\alpha \mathrm{p}} \nu^0_\alpha \right) \right]. \tag{S36}$$

Hence, only gradients of the chemical potentials appear in the driving forces, so we can further simplify the formula. In the one-dimensional and electroneutral case, the gradient of the pressure is a function of the volume ratio $J$ only (cf. eq. (S26)), which in the polymer volume dominance assumption is constant, so the pressure gradient vanishes, $\mathrm{grad}(p) = 0$. With no magnetic fields and in the electroneutral case,

$$\mathrm{grad} \left( \boldsymbol{\mathcal{E}} \cdot \boldsymbol{D} + \boldsymbol{\mathcal{H}} \cdot \boldsymbol{B} \right) = -2\rho^\mathrm{F} \cdot \mathrm{grad}(\phi) = 0. \tag{S37}$$

For the further simplification, we consolidate all constant terms of the chemical potential,

$$\mu_\alpha = \mu^\mathrm{const}_\alpha + RT \log \left( \nu^0_\alpha c_\alpha \right). \tag{S38}$$

The constant part of the chemical potential is given by $\mu^\mathrm{const}_\alpha = M_\alpha \varphi^0_\alpha + \nu^0_\alpha p - \frac{1}{6} \left( \boldsymbol{\mathcal{E}} \cdot \boldsymbol{D} + \boldsymbol{\mathcal{H}} \cdot \boldsymbol{B} \right) + RT \left( 1 - \delta_{\alpha \mathrm{p}} \right) \cdot \left( 1 + \xi_{\alpha \mathrm{p}} \nu^0_\alpha \right)$. To finalize the reduction of the chemical potential, we introduce the activity coefficients $f_\alpha$ to capture deviations from the ideal behaviour (with volume fractions $\nu_\alpha c_\alpha$)

$$\mu_\alpha = \mu^\mathrm{const}_\alpha + RT \log \left( f_\alpha c_\alpha \right). \tag{S39}$$

This reproduces the form for the chemical potentials as found in concentrated solution theory.

Next, we assume that $\rho_\mathrm{p} \approx \rho$, and that the molar masses of the non-polymer species $\alpha \neq \mathrm{p}$ are much smaller than the polymer molar mass $M_\alpha \ll M_\mathrm{p}$. With this, the reference change matrices S11 between the center-of-mass and the polymer reference frames simplify to unity: $A_{\alpha\beta} = \delta_{\alpha\beta} = A^{-1}_{\alpha\beta}$. Since the total mass is given by the polymer species, the two reference frames are identical, as are the respective convection velocities $\boldsymbol{v} = \sum_{\alpha=1}^{\mathrm{N}} \frac{\rho_\alpha}{\rho} \boldsymbol{v}_\alpha = \frac{\rho_\mathrm{p}}{\rho} \boldsymbol{v}_\mathrm{p} = \boldsymbol{v}_\mathrm{p}$. The driving forces in the polymer frame (see eq. (S14)) reduce to the gradients of the electro-chemical potentials

$$\boldsymbol{\mathcal{F}}^\mathrm{el,p}_\beta = \mathrm{grad} \left( \mu^\mathrm{el}_\beta \right) = \frac{RT}{c_\alpha} \cdot \mathrm{TDF}_\alpha \cdot \mathrm{grad} \left( c_\alpha \right), \tag{S40}$$

with the thermodynamic factor $\mathrm{TDF}_\alpha = 1 + \frac{\partial \log(f_\alpha)}{\partial \log(c_\alpha)}$ of species $\alpha$.

In concentrated solution theory, the molar fluxes are expressed in terms of gradients of the chemical potentials and the current density, while the current density is expressed in terms of the gradients of the chemical and "electrical potentials".[5,7] We note, however, that the term "electrical potential" in this context corresponds to the potential measured by a reference electrode.[6] In our modelling framework, we introduce the chemo-electrical potentials $\varphi_\alpha = \mu^{\mathrm{el}}_\alpha/(Fz_\alpha)$, which correspond to the "electrical potentials" in CST.[8] In the PEO/LiTFSI electrolyte of Steinrück et al. the Li-metal reference electrode measures the chemo-electrical potential $\varphi$ of the Li cations,

$$\mathrm{grad}\,(\varphi) = \mathrm{grad}\,(\phi) + \frac{\boldsymbol{\mathcal{F}}_2^{\mathrm{V}}}{F\tilde{z}_2^{\mathrm{V}}}. \tag{S41}$$

The molar flux densities (eqn. 24) of our transport theory are then given by

$$\boldsymbol{N}_\alpha^{\mathrm{p}} = -\sum_{\beta=1}^{\mathrm{N}} \mathcal{L}_{\alpha\beta}^{\mathrm{p}} \cdot \left( \boldsymbol{\mathcal{F}}_\beta^{\mathrm{p}} - \frac{\tilde{z}_\beta^{\mathrm{p}}}{z_+}\mathrm{grad}\,(\mu_+) \right) - \sum_{\beta=1}^{\mathrm{N}} \mathcal{L}_{\alpha\beta}^{\mathrm{p}} F \tilde{z}_\beta^{\mathrm{p}} \cdot \mathrm{grad}\,(\varphi) - \mathcal{L}_{\beta T}^{\mathrm{p}} \cdot \mathcal{F}_T^{\mathrm{p}}, \tag{S42}$$

with effective polymer-frame charge numbers $\tilde{z}_\beta^{\mathrm{p}} = \sum_{\alpha=2}^{\mathrm{N}} (z_\beta - M_\beta/M_{\mathrm{p}} \cdot z_{\mathrm{p}}) A_{\beta\alpha}^{-1}$. Furthermore, the thermodynamic forces with respect to the polymer-frame, $\boldsymbol{\mathcal{F}}_\beta^{\mathrm{p}} = \sum_{\alpha=2}^{\mathrm{N}} (\boldsymbol{\mathcal{F}}_\alpha - M_\alpha/M_{\mathrm{p}} \cdot [\boldsymbol{\mathcal{F}}_{\mathrm{mech}} + \rho s/c_{\mathrm{p}} \cdot \boldsymbol{\mathcal{F}}_{\mathrm{T}} + \boldsymbol{\mathcal{F}}_{\mathrm{p}}]) A_{\alpha\beta}^{-1}$ have no contributions from the electric potential $\boldsymbol{\mathcal{F}}_\alpha = \mathrm{grad}\,(\mu_\alpha)$. For the case of the polymer electrolyte system used by Steinrück et al., which consists of three distinct species $\alpha \in \{\mathrm{p}, +, -\}$ with $z_{\mathrm{p}} = 0$, $z_+ = +1$, $z_- = -1$, in electroneutral state, and using the two assumptions described above, the molar fluxes read (no thermal gradients),

$$\begin{aligned} \boldsymbol{N}_\alpha^{\mathrm{p}} &= -\mathcal{L}_{\alpha-}^{\mathrm{p}} \cdot (\mathrm{grad}\,(\mu_-) + \mathrm{grad}\,(\mu_+)) - \sum_{\beta=1}^{\mathrm{N}} \mathcal{L}_{\alpha\beta}^{\mathrm{p}} F z_\beta \cdot \mathrm{grad}\,(\varphi) \\ &= -\mathcal{L}_{\alpha-}^{\mathrm{p}} \cdot 2\frac{RT}{c_+}\left(1 + \frac{\partial \log(f)}{\partial \log(c_+)}\right) \cdot \mathrm{grad}\,(c_+) - \sum_{\beta=1}^{\mathrm{N}} \mathcal{L}_{\alpha\beta}^{\mathrm{p}} F z_\beta \cdot \mathrm{grad}\,(\varphi)\,. \end{aligned} \tag{S43}$$

Here, $f^2 = f_+ f_-$ is the combined activity coefficient of the cation and anion. The current density is given by the charge-weighted sum,

$$\boldsymbol{\mathcal{J}}^{\mathrm{p}} = \sum_{\alpha=2}^{\mathrm{N}} F z_\alpha \boldsymbol{N}_\alpha^{\mathrm{p}} = -\sum_{\alpha=1}^{\mathrm{N}} F z_\alpha \mathcal{L}_{\alpha-}^{\mathrm{p}} \cdot 2\frac{RT}{c}\left(1 + \frac{\partial \log(f)}{\partial \log(c_+)}\right) \cdot \mathrm{grad}\,(c_+) - \sum_{\alpha,\beta=2}^{\mathrm{N}} F^2 z_\alpha \mathcal{L}_{\alpha\beta}^{\mathrm{p}} z_\beta \cdot \mathrm{grad}\,(\phi)\,. \tag{S44}$$

Expressing the molar fluxes and the current density of CST in a similar form with the gradients of the cation concentration and the chemo-electrical potential and comparing the coefficients yields for the Onsager coefficients,

$$\mathcal{L}_{\alpha\beta}^{\mathrm{p}} = \frac{1}{2}\frac{\mathcal{D}}{RT}\frac{c_{\mathrm{T}} c_+}{c_{\mathrm{p}}} + \frac{t_\alpha t_\beta \kappa}{F^2 z_\alpha z_\beta}, \tag{S45}$$

with the diffusion coefficient $\mathcal{D}$, the transference numbers $t_\alpha$, and the ionic conductivity $\kappa$. These are all modelled using concentration-dependent parameters from Steinrück et al.[5], and interpolated linearly, as is the thermodynamic factor $1 + \frac{\partial \log(f)}{\partial \log(c_+)}$. The total concentration is $c_{\mathrm{T}} = \sum_{\alpha=1}^{\mathrm{N}} c_\alpha$.

## F. Volume-frame

In this section, we discuss the alternative frame of reference defined by the volume averaged convection velocity. Here, we state all relevant results, and refer to our publications Refs.[2,4] for more details.

The volume-averaged velocity is given by $\boldsymbol{v}_{\mathrm{V}} = \sum_{\alpha=1}^{\mathrm{N}} \nu_\alpha c_\alpha \boldsymbol{v}_\alpha$. This gives rise to molar fluxes $\boldsymbol{N}_\alpha^{\mathrm{V}} = c_\alpha(\boldsymbol{v}_\alpha - \boldsymbol{v}_{\mathrm{V}})$, which appear in the continuity equation

$$\frac{\partial}{\partial t} c_\alpha = -\mathrm{div}\left(\boldsymbol{N}_\alpha^{\mathrm{V}}\right) - \mathrm{div}\,(c_\alpha \boldsymbol{v}_{\mathrm{V}})\,. \tag{S46}$$

The molar fluxes fulfill $\sum_{\alpha=1}^{N} \nu_\alpha \boldsymbol{N}_\alpha^{V} = 0$. In the incompressible limit $\nu_\alpha = \nu_\alpha^0$ we find

$$\operatorname{div}(\boldsymbol{v}_{V}) = 0. \tag{S47}$$

The molar fluxes can be transformed between two frames of reference $\Psi$ and $\tilde{\Psi}$ via

$$\boldsymbol{N}_\alpha^{\Psi} = \sum_{\beta=2}^{N} A_{\alpha\beta}^{\Psi\tilde{\Psi}} \cdot \boldsymbol{N}_\beta^{\tilde{\Psi}}, \tag{S48}$$

where $\Psi$ and $\tilde{\Psi}$ denote two frames of reference, e.g. the center-of-mass frame, the volume frame, or the polymer frame. Note that the transformation matrices $\boldsymbol{A}^{\Psi\tilde{\Psi}} = \left(\boldsymbol{A}^{\tilde{\Psi}\Psi}\right)^{-1}$. For the special cases of the frames of reference used in this publication, we have

$$A_{\alpha\beta}^{\mathrm{VM}} = \delta_{\alpha\beta} - c_\alpha \left(\nu_\beta - \frac{M_\beta}{M_{\mathrm{p}}}\nu_{\mathrm{p}}\right), \qquad A_{\alpha\beta}^{\mathrm{MV}} = \delta_{\alpha\beta} - \frac{c_\alpha}{\rho}\left(M_\beta - \frac{\nu_\beta}{\nu_{\mathrm{p}}}M_{\mathrm{p}}\right), \tag{S49}$$

$$A_{\alpha\beta}^{\mathrm{Vp}} = \delta_{\alpha\beta} - c_\alpha \nu_\beta, \qquad A_{\alpha\beta}^{\mathrm{pV}} = \delta_{\alpha\beta} + \frac{c_\alpha \nu_\beta}{c_{\mathrm{p}} \nu_{\mathrm{p}}}. \tag{S50}$$

The transformations between the polymer- and center-of-mass frames are stated in eq. (S11).

In the electro-neutral case, the components of the symmetric diffusion coefficient matrix are given by

$$\mathcal{D}_{\alpha\beta}^{V} = \mathcal{L}_{\alpha\beta}^{V} - \frac{t_\alpha^{V} t_\beta^{V} \kappa^{V}}{F^2 \tilde{z}_\alpha^{V} \tilde{z}_\beta^{V}}, \tag{S51}$$

with $\tilde{z}_\alpha^{V} = z_\alpha - \nu_\alpha/\nu_{\mathrm{p}} \cdot z_{\mathrm{p}}$. The transference numbers $t_\alpha^{V}$ and the ionic conductivity $\kappa^{V}$ are given by

$$t_\alpha^{V} = \frac{F^2 \tilde{z}_\alpha^{V}}{\kappa^{V}} \sum_{\beta=2}^{N} \tilde{z}_\beta^{V} \mathcal{L}_{\alpha\beta}^{V}, \qquad \kappa^{V} = F^2 \sum_{\alpha,\beta=2}^{N} \tilde{z}_\alpha^{V} \mathcal{L}_{\alpha\beta}^{V} \tilde{z}_\beta^{V}. \tag{S52}$$

Similar to section S1 E, we use the chemo-electrical potential $\operatorname{grad}(\varphi) = \operatorname{grad}(\phi) + \boldsymbol{\mathcal{F}}_2^{V}/F\tilde{z}_2^{V}$, and the reduced driving forces $\tilde{\boldsymbol{\mathcal{F}}}_\beta^{V} = \boldsymbol{\mathcal{F}}_\beta^{V} - \tilde{z}_\beta^{V}/\tilde{z}_2^{V} \cdot \boldsymbol{\mathcal{F}}_2^{V}$ to express the current density and the molar fluxes in the volume frame:

$$\boldsymbol{\mathcal{J}}^{V} = -\kappa^{V} \cdot \operatorname{grad}(\varphi) - \sum_{\beta=3}^{N} \frac{t_\beta^{V} \kappa^{V}}{F \tilde{z}_\beta^{V}} \cdot \tilde{\boldsymbol{\mathcal{F}}}_\beta^{V}, \tag{S53}$$

$$\boldsymbol{N}_\alpha^{V} = \frac{t_\alpha^{V}}{F z_\alpha} \cdot \boldsymbol{\mathcal{J}}^{V} - \sum_{\beta=3}^{N} \mathcal{D}_{\alpha\beta}^{V} \cdot \tilde{\boldsymbol{\mathcal{F}}}_\beta^{V}. \tag{S54}$$

## S2. SIMULATION

### A. Parameters

#### 1. *PEO/LiTFSI*

The first investigated polymer electrolyte in the symmetric Li/electrolyte/Li cell has a thickness of 3 mm and consists of a PEO polymer host (molecular weight 600 000 kg mol$^{-1}$) with a LiTFSI salt (ratio of ethylene oxide monomer units to Li cations: EO:Li$^+$=10:1). After an initial linear ramp-up during the first second, the voltage difference of the electrodes is held constant at $\Delta U$=0.3 V over the total simulation time of 1000 min. At a constant temperature of $T$=90 °C, the shear and bulk moduli of PEO (solvated by LiTFSI) are given by $G_{\mathrm{p}}$=8 MPa and $K_{\mathrm{p}}$=3 MPa[9–11]. The constant partial molar volumes for the three species are $\nu_{\mathrm{p}}$=, $\nu_{\mathrm{Li}}$= and $\nu_{\mathrm{TFSI}}$=.

Except for the Flory-Huggins interaction parameters, the polymer electrolyte is fully parametrized from literature. We obtained the current density shown in fig. 4, which shows a relatively good agreement with the current density from CST, with the Flory-Huggins interaction parameters $\chi_{\mathrm{LiTFSI}}=-6$, $\chi_{\mathrm{Lip}}=-20$ and $\chi_{\mathrm{TFSIp}}=-15$.[12] Note that,

| Numerical parameter | Value for PEO/LiTFSI | Value for SIC/EC |
|---|---|---|
| Matlab ODE solver | ode15s | ode15s |
| Absolute tolerance | $10^{-6}$ | $10^{-9}$ |
| Relative tolerance | $10^{-6}$ | $10^{-9}$ |
| Number of grid elements | $i_{\max} = 100$ | $i_{\max} = 100$ |

TABLE S1. Numerical parameters for the implementation of the one-dimensional transport model.

for notational purposes, we introduced the Flory-Huggins interaction parameters in the free energy density (eq. (30)) in a slightly different form, $\xi_{\alpha\beta} = \chi_{\alpha\beta}/\nu_\alpha = \chi_{\beta\alpha}/\nu_\beta$. Since $\chi_{+\mathrm{p}} < \chi_{+\mathrm{s}}$, these Flory-Huggins interaction parameters indicate a higher tendency of the $Li^+$-ions to coordinate to the polymer species than to the $TFSI^-$-ions. This corresponds to results from molecular dynamics simulations, in which the $Li^+$-ions almost exclusively coordinate to oxygen atoms from EO monomers.[13]

### *2. SIC/EC*

The second investigated polymer electrolyte consists of a newly developed single-ion conducting polymer (SIC), solvated with ethylene carbonate (EC) at a weight percentage of 50%.[14] The geometrical setup, the protocol for the applied voltage and the surface reaction rates are identical to the first investigated polymer electrolyte. Since no measurements of the elastic properties of this polymer were published, the elastic modulus is assumed to be similar to that of Nafion at a relative humidity of 50% with $E_\mathrm{p} = 249\,\mathrm{MPa}$.[15] The partial molar volumes for the three species are $\nu_\mathrm{p}$=, $\nu_\mathrm{Li}$= and $\nu_\mathrm{EC}$=. For the Flory-Huggins parameters we chose $\chi_{23} = -5$, $\chi_{21} = -20$ and $\chi_{31} = -10$.

## B. Numerical Methods

In this section we outline the numerical methods used for the potentiostatic discharge simulations of the two different polymer electrolyte materials as presented in sections III B and IV B. We implement the one-dimensional transport models eqs. (45) to (47) and eqs. (50) to (52) in Matlab using the finite-volume scheme. In this scheme, the physical quantities like the molar concentrations $c_\alpha$ are defined inside volume elements $V_i$ with $i = 1, ..., i_{\max}$, while fluxes of physical quantities like the current density $\boldsymbol{\mathcal{J}}^\mathrm{p}$, the molar fluxes $\boldsymbol{N}_\alpha^\mathrm{p}$ or the convection velocity $\boldsymbol{v}_\mathrm{p}$ are defined on the boundaries $B_i$ with $i = 0, ..., i_{\max}$, between two adjacent volume elements. As boundary conditions at the interfaces $B_0$ and $B_{i_{\max}}$ between electrolyte and electrode we assume all flux-like quantities to vanish. This means that at $x$=$B_0$ and $x$=$B_{i_{\max}}$ the current density $\boldsymbol{\mathcal{J}}^\Psi(x)$, the species molar fluxes $\boldsymbol{N}_\alpha^\Psi(x)$ and the convection velocity $\boldsymbol{v}_\Psi(x)$ vanish for all reference frames $\Psi$. The motion of lithium ions from the electrodes to the electrolyte is included into the system of differential equations by the reaction rate

$$r_\mathrm{Li}(V_i) = \frac{j_\mathrm{elde,l}}{F z_\mathrm{Li}} \cdot \delta_{i,1} + \frac{j_\mathrm{elde,r}}{F z_\mathrm{Li}} \cdot \delta_{i,i_{\max}}, \tag{S55}$$

where $\delta$ denotes the Kronecker delta and $j_\mathrm{elde,l/r}$ are the current densities provided by the left or right electrode, respectively. These are modelled using a Butler-Volmer Ansatz

$$j_\mathrm{elde,l/r} = j_0 \cdot \left[ \exp\left( \frac{\alpha F}{RT} \left( \varphi_\mathrm{elde,l/r} - \varphi_\mathrm{elyte}(V_1/V_{i_{\max}}) \right) \right) - \exp\left( -\frac{(1-\alpha)\,F}{RT} \left( \varphi_\mathrm{elde,l/r} - \varphi_\mathrm{elyte}(V_1/V_{i_{\max}}) \right) \right) \right], \tag{S56}$$

with the exchange current density $j_0 = 0.5\,\mathrm{mA\,cm^{-2}}$ [6] and the symmetry factor $\alpha = 0.5$. The electrolyte potential $\varphi_\mathrm{elyte}(V_i)$ is the chemo-electrical potential of the electrolyte in volume element $V_i$ at the electrode interface (see eq. (S41)). The potential $\varphi_\mathrm{elde,l/r}$ of the left/right electrode, which for the lithium metal electrode is simply the applied voltage, is not dependent on the state-of-charge (*cf.* Steinrück *et al.*[5]). Table S1 lists the numerical details used for the simulations.

## C. Thermodynamic transport contributions

In this section, we compare the main differences between our derived transport model and the use of concentrated solution theory (CST) for the sample case of the PEO/LiTFSI polymer electrolyte, as presented in section III.

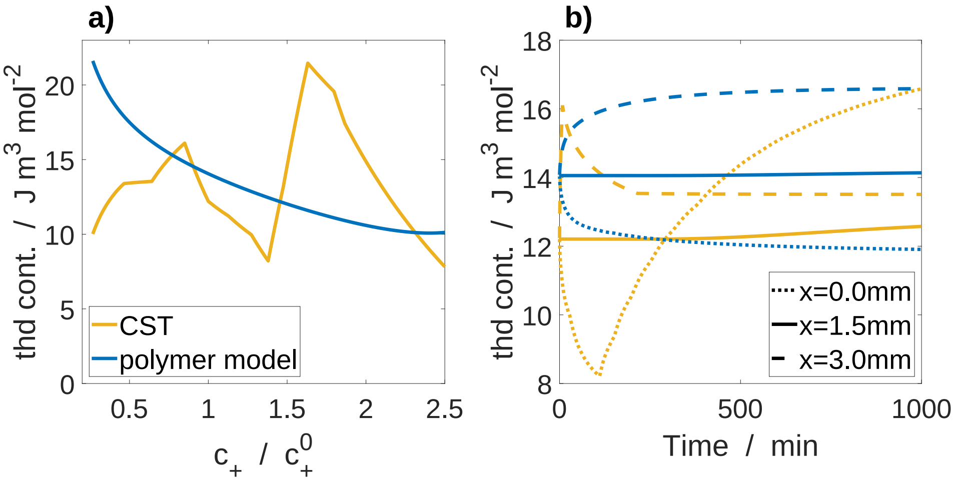


FIG. S1. The thermodynamic transport contributions for CST (yellow) and our derived transport model for polymer electrolytes (blue). The left graph a) depicts the thermodynamic transport contributions over the concentration range of $c_{\mathrm{Li}}$. In the right graph b), the thermodynamic transport contributions at distinct locations in the electrolyte (distinct plot styles) are depicted for both CST (yellow) and our polymer model (blue).

In our derived transport model, the contributions to species and charge transport can be split into two categories: kinetic and thermodynamic, as described in section II A. The kinetic transport contributions are comprised in the Onsager coefficients $\mathcal{L}$. For the potentiostatic simulations of the PEO/LiTFSI electrolyte in section III, we parametrize these Onsager coefficients with the transport parameters used for the CST simulations by Steinrück *et al.*.[5] The details of this parametrization are described in section S1 E. Using this procedure, the kinetic transport contributions of our model and CST are identical. Therefore, we focus on the thermodynamic transport contributions to work out the differences of the two models.

The current density in our transport theory is given by

$$\boldsymbol{\mathcal{J}}^{\mathrm{p}} = -\kappa^{\mathrm{p}} \cdot \mathrm{grad}\,(\varphi) + \frac{(1 - t^{\mathrm{p}}_{\mathrm{Li}})\,\kappa^{\mathrm{p}}}{F z_{\mathrm{Li}}} \cdot \tilde{\boldsymbol{\mathcal{F}}}^{\mathrm{p}}_{3}, \tag{S57}$$

while the current density used in CST has the form

$$\boldsymbol{\mathcal{J}}^{\mathrm{p}} = -\kappa^{\mathrm{p}} \cdot \mathrm{grad}\,(\varphi) + 2\frac{(1 - t^{\mathrm{p}}_{\mathrm{Li}})\,\kappa^{\mathrm{p}}}{F z_{\mathrm{Li}}}\frac{RT}{c_{\mathrm{Li}}}\left(1 + \frac{\partial \log f}{\partial \log c_{\mathrm{Li}}}\right) \cdot \mathrm{grad}\,(c_{\mathrm{Li}})\,. \tag{S58}$$

The term in brackets $1+\frac{\partial \log f}{\partial \log c_{\mathrm{Li}}}$ is commonly referred to as "thermodynamic factor", where $f$ is the activity coefficient used in the chemical potential to describe behaviour deviating from that of ideal gases (see section S1 E). By comparing the two expressions eq. (S57) and eq. (S58), we find the respective expressions corresponding to the thermodynamic transport contributions:

$$\frac{\tilde{\boldsymbol{\mathcal{F}}}^{\mathrm{p}}_{3}}{\mathrm{grad}\,(c_{\mathrm{Li}})} \quad \text{and} \quad 2\frac{RT}{c_{\mathrm{Li}}}\left(1 + \frac{\partial \log f}{\partial \log c_{\mathrm{Li}}}\right). \tag{S59}$$

In a perfect match of the two models, these expressions would be equal. However, we obtained the left side corresponding to our transport model from fundamental physical considerations, while the right side corresponding to CST was fitted to experimental results. Figure S1 depicts the thermodynamic transport contributions for both CST (yellow) and our transport model for polymer electrolytes (blue). Figure S1 a) depicts the thermodynamic transport contributions over the relevant range of the Li-cation concentration $c_{\mathrm{Li}}$. For CST, a table of specific values for the thermodynamic transport contributions are given for the respective values of $c_{\mathrm{Li}}$, where we have a used a linear interpolation for the concentrations in between. In contrast, the thermodynamic transport contribution for our polymer model is derived from the driving forces and is a smooth function of $c_{\mathrm{Li}}$. The CST values show two peaks at $c_{\mathrm{Li}}$=0.85 $c^0_{\mathrm{Li}}$=1590 mol m$^{-3}$ and $c_{\mathrm{Li}}$=1.63 $c^0_{\mathrm{Li}}$=3050 mol m$^{-3}$, while dropping to its lowest value at $c_{\mathrm{Li}}$=1.38 $c^0_{\mathrm{Li}}$=2580 mol m$^{-3}$. The CST values also decrease for $c_{\mathrm{Li}}\rightarrow 0$. The thermodynamic contribution for our polymer model shows an increase towards lower concentrations $c_{\mathrm{Li}}$. The dominating aspect for this behaviour is given by the entropic contributions to the free energy eq. (30), which provide a factor $1/c_{\mathrm{Li}}$ in the driving forces. For larger lithium concentrations $c_{\mathrm{Li}}$, the thermodynamic

contribution decreases, until at $c_{\mathrm{Li}}{\approx}2.5\,c^0_{\mathrm{Li}}$, it starts to slowly rise again. Since the Li-cation concentration is strongly coupled to the TFSI-anion concentration, an increase in $c_{\mathrm{Li}}$ means a larger volume fraction of cations and anions. The polymer responds by stretching and thus increasing its volume ratio $J$. This results in a large mechanical energy in the polymer, which becomes the dominating aspect for the thermodynamic transport contributions for large concentrations $c_{\mathrm{Li}}{>}2.5\,c^0_{\mathrm{Li}}$.

The thermodynamic transport contributions for both models are relatively close to each other in the range from $c_{\mathrm{Li}}{\approx}0.7\,c^0_{\mathrm{Li}}{=}1309\,\mathrm{mol\,m^{-3}}$ to $c_{\mathrm{Li}}{\approx}1.5\,c^0_{\mathrm{Li}}{=}2805\,\mathrm{mol\,m^{-3}}$. For small concentrations $c_{\mathrm{Li}}{<}0.7\,c^0_{\mathrm{Li}}$, the two models diverge strongly. While for CST the thermodynamic contribution decreases for $c_{\mathrm{Li}} \to 0$, it increases for our polymer model. This could be a hint for effects relevant at small cation concentrations that are not included in our model. For larger concentrations $c_{\mathrm{Li}}{>}1.5\,c^0_{\mathrm{Li}}$, the two models also differ significantly. CST shows a steep peak, followed by a decrease. However, this decrease is a result of the extrapolation of the data provided by Steinrück *et al.*,[5] in which the largest concentration value is $c_{\mathrm{Li}}{=}2.0\,c^0_{\mathrm{Li}}$.

Figure S1 b) depicts the specific values for the thermodynamic transport contributions during the galvanostatic simulation at three distinct locations in the electrolyte for both CST (yellow) and our polymer model (blue). The three locations are next to the positive electrode at $x{=}0.0\,\mathrm{mm}$ (dotted lines), at the center of the electrolyte at $x{=}1.5\,\mathrm{mm}$ (solid line), and next to the negative electrode at $x{=}3.0\,\mathrm{mm}$ (dashed lines).

The thermodynamic contribution at $x{=}1.5\,\mathrm{mm}$ (solid lines) does not change significantly over the whole simulation run for both models, since the Li-cation concentration $c_{\mathrm{Li}}$ remains fairly constant at the center of the electrolyte. In the viccinity of the positive electrode at $x{=}0.0\,\mathrm{mm}$ (dotted lines), the concentration $c_{\mathrm{Li}}$ increases with time due to concentration polarization, as shown in fig. 5. For CST, the thermodynamic contribution follows the concentration as depicted in Figure S1 a), first dropping until reaching the minimum at $c_{\mathrm{Li}}{=}1.38\,c^0_{\mathrm{Li}}$ at a simulation time of $t \approx 110\,\mathrm{min}$, then increasing again. In contrast, the thermodynamic contribution for our polymer model shows a monotonic fall over the whole duration of the simulation. At the negative electrode at $x{=}3.0\,\mathrm{mm}$, the Li-cation concentration $c_{\mathrm{Li}}$ decreases with time. The value for CST increases sharply during the first 8 min (dashed line), which is followed by a slower descent. Our polymer model shows a steady increase, which flattens off with increasing time.

For nearly all times, the thermodynamic contributions of our polymer model are larger than that of CST, except for the location near the positive electrode $x{=}0.0\,\mathrm{mm}$ (dotted lines) for times $t{>}290\,\mathrm{min}$. Since a larger thermodynamic contribution leads to a higher diffusion flux with a given concentration gradient, our polymer model results in a slightly smaller overall concentration polarization, as can be seen in fig. 5.

## S3. STEADY STATE AND POLYMER DEFORMATION

In this section, we focus on the stationary state of the as-described SIC-based polymer-electrolyte (see section IV C) while an constant current is applied, and present an analytical discussion for the resulting polymer deformation.

In the stationary state, the system remains constant over time, so all time derivatives vanish. The equation of motion of species $\alpha$ in stationary state becomes:

$$0 = \frac{\partial\left(\epsilon c_\alpha\right)}{\partial t} = -\mathrm{div}\left(\epsilon^\beta \boldsymbol{N}^{\mathrm{V}}_\alpha\right) - \mathrm{div}\left(\epsilon c_\alpha \boldsymbol{v}_{\mathrm{V}}\right) + r_\alpha. \tag{S60}$$

In the one-dimensional case, we can integrate this equation. This gives for the single terms, using the appropriate boundary conditions at the electrode/electrolyte interface $x{=}0$ (*cf.* section S2 B):

$$\int_0^x \mathrm{div}\left(\epsilon^\beta N^{\mathrm{V}}_\alpha\right)(x')\,dx' = \epsilon^\beta N^{\mathrm{V}}_\alpha(x) - \epsilon^\beta N^{\mathrm{V}}_\alpha(0) = \epsilon^\beta N^{\mathrm{V}}_\alpha(x)\,, \tag{S61}$$

$$\int_0^x \mathrm{div}\left(\epsilon c_\alpha v_{\mathrm{V}}\right)(x')\,dx' = \epsilon c_\alpha(x)\,v_{\mathrm{V}}(x) - \epsilon c_\alpha(0)\,v_{\mathrm{V}}(0) = \epsilon c_\alpha(x)\,v_{\mathrm{V}}(x)\,, \tag{S62}$$

$$\int_0^x r_{\mathrm{Li}}(x')dx' = \frac{j_{\mathrm{elde,l}}}{F z_{\mathrm{Li}}}. \tag{S63}$$

In contrast to the discrete formulation eq. (S55) of the reaction rate $r_{\mathrm{Li}}$, we use here the continuous formulation $r_{\mathrm{Li}}(x){=}\frac{j_{\mathrm{elde,l}}}{F z_{\mathrm{Li}}}\cdot\delta(x)$, where $\delta$ denotes the delta distribution. Analogously, we obtain values for $\boldsymbol{v}_{\mathrm{V}}$ and $J^{\mathrm{V}}$ by integration of eqs. (50) and (52):

$$\epsilon v_{\mathrm{V}}(x) = \frac{\nu_{\mathrm{Li}}}{F z_{\mathrm{Li}}} j_{\mathrm{elde,l}} \tag{S64}$$

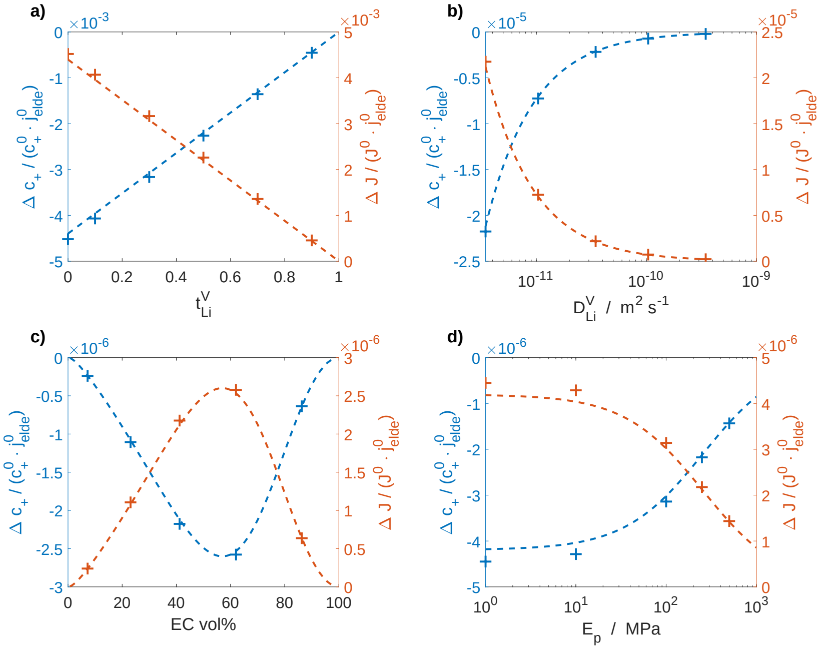


FIG. S2. These four graphs depict the resulting polymer deformation and concentration difference across the electrolyte for variations in single parameters. The dashed lines denote the results obtained analytically from eq. (S67). The crosses denote the numerical results obtained from the transport model to validate the analytical formula.

$$\epsilon^{\beta}\mathcal{J}^{\mathrm{V}}(x) = j_{\mathrm{elde,l}} \tag{S65}$$

Using these results and inserting the explicit expression for the volume-frame solvent flux eq. (S54), we obtain a constraint for the stationary state from eq. (S60) for $\alpha = \mathrm{Li}$:

$$0 = -\frac{t_{\mathrm{Li}}^{\mathrm{V}}}{F z_{\mathrm{Li}}} j_{\mathrm{elde,l}} + \epsilon^{\beta} D_{\mathrm{Li}}^{\mathrm{V}} \tilde{\mathcal{F}}_{\mathrm{TFSI}}^{\mathrm{V}} - \frac{\nu_{\mathrm{Li}} c_{\mathrm{Li}}}{F z_{\mathrm{Li}}} j_{\mathrm{elde,l}} + j_{\mathrm{elde,l}}. \tag{S66}$$

We develop the driving forces in terms of the gradient of the lithium concentration $\tilde{\mathcal{F}}_{\mathrm{TFSI}}^{\mathrm{V}} = \tilde{\mathcal{F}}_{\mathrm{TFSI},c_{\mathrm{Li}}}^{\mathrm{V}} \cdot \mathrm{grad}\,(c_{\mathrm{Li}})$. From the connection of $c_{\mathrm{Li}}$ and $J$ (see eq. (S19)) we obtain the gradient of the volume ratio by using the chain-rule for derivatives $\mathrm{grad}\,(c_{\mathrm{Li}}) = \frac{\partial c_{\mathrm{Li}}}{\partial J} \cdot \mathrm{grad}\,(J)$. The expression for the polymer deformation during steady state is given by:

$$\mathrm{grad}\,(J) = -\frac{1 - t_{\mathrm{Li}}^{\mathrm{V}} - c_{\mathrm{Li}}\nu_{\mathrm{Li}}}{F z_{\mathrm{Li}} \cdot \epsilon^{\beta} \mathcal{D}_{\mathrm{Li}}^{\mathrm{V}} \cdot \frac{\partial c_{\mathrm{Li}}}{\partial J}} \cdot \left(\tilde{\mathcal{F}}_{\mathrm{TFSI},c_{\mathrm{Li}}}^{\mathrm{V}}\right)^{-1} \cdot j_{\mathrm{elde,l}} = -\Omega \cdot j_{\mathrm{elde,l}} \tag{S67}$$

We have combined the prefactors into a single factor $\Omega$ for ease of notation. This single factor can be split up into a "transport factor" $\Xi$ and a "material factor" $\Theta$:

$$\Xi = \frac{1 - t_{\mathrm{Li}}^{\mathrm{V}} - c_{\mathrm{Li}}\nu_{\mathrm{Li}}}{F z_{\mathrm{Li}} \cdot \epsilon^{\beta} \mathcal{D}_{\mathrm{Li}}^{\mathrm{V}} \cdot \frac{\partial c_{\mathrm{Li}}}{\partial J}}, \qquad \Theta = \left(\tilde{\mathcal{F}}_{\mathrm{TFSI},c_{\mathrm{Li}}}^{\mathrm{V}}\right)^{-1}. \tag{S68}$$

As can be seen, the "transport factor" $\Omega$ is a function mainly of the transport parameters $t_{\mathrm{Li}}^{\mathrm{V}}$ and $\mathcal{D}_{\mathrm{Li}}^{\mathrm{V}}$, while $c_{\mathrm{Li}}\nu_{\mathrm{Li}}$ is negligible. The partial derivative is given by $\frac{\partial c_{\mathrm{Li}}}{\partial J} = \frac{z_{\mathrm{p}}}{z_{\mathrm{Li}}\nu_{\mathrm{p}} J^2}$. The "material factor" $\Theta$, as the inverse of the reduced driving force $\tilde{\mathcal{F}}_{\mathrm{TFSI},J}^{\mathrm{V}}$, is a function of material parameters like *e.g.* the polymer elastic modulus $E_{\mathrm{p}}$, the initial composition given by the EC solvent volume ratio, the partial molar volumes $\nu_{\alpha}$ or the Flory-Huggins parameters $\xi_{\alpha\beta}$, but not of the transport parameters.

In the following, the results of eq. (S67) are given. As in the main text section IV C, we vary several parameters and compare the resulting deformations of the polymer. Figure S2 shows the lithium cation concentration difference (blue, left axis) and the polymer deformation (orange, right axis) obtained from the analytical formula eq. (S67) (dashed lines) and from numerical galvanostatic discharge simulations (crosses) to validate the analytical formula. The measure

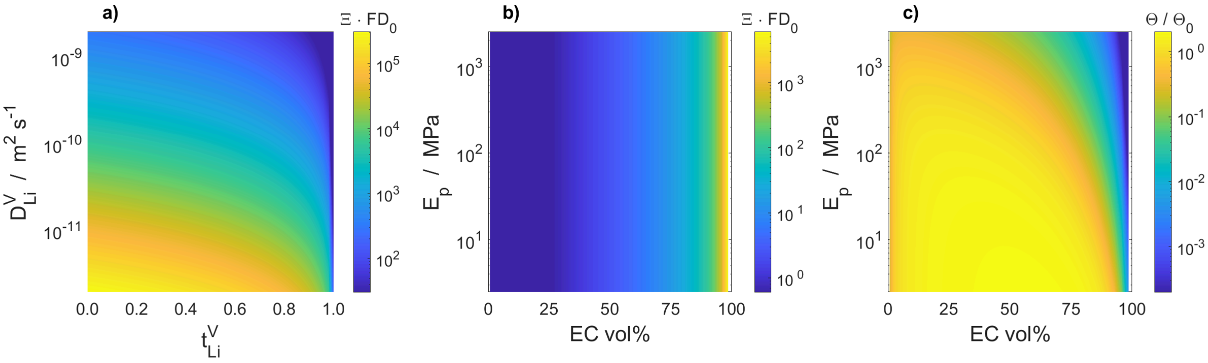


FIG. S3. The values for the transport and material factors eq. (S68) are shown for ranges of pairs of transport and material parameters. The resulting polymer deformation is depicted in fig. 7 of the main text.

for the deformation of the polymer matrix is given by the normalized variation of $J$ from the left electrode to the right electrode, *e.g.* $\Delta J = (J(x=L) - J(x=0))/J^0$, divided by the non-dimensionalized current density $j^0_{\mathrm{elde,l}}$=$j_{\mathrm{elde,l}}/j_0$, with the exchange current density $j_0$ as in eq. (S56). The concentration difference is the difference of the lithium cation concentrations at the left and right electrodes, divided by the non-dimensionalized current density $j^0_{\mathrm{elde,l}}$. Since the volume ratio behaves inversely to the polymer and lithium concentrations $J \propto \frac{1}{c_{\mathrm{p}}} \propto \frac{1}{c_{\mathrm{Li}}}$, the concentration difference has a different sign than the polymer deformation, but behaves similarly. Hence, we will only discuss the results for the polymer deformation in the following.

In fig. S2 a) to d), one parameter is varied, while the respective others are held constant. The four parameters and their reference values are the lithium transference number $t^{\mathrm{V}}_{\mathrm{Li}}$=1, the lithium diffusion coefficient $D^{\mathrm{V}}_{\mathrm{Li}}$=$1.94 \times 10^{-10}\,\mathrm{m^2\,s^{-1}}$, the volume ratio of the EC solvent EC vol%=41%, and the elastic modulus of polymer $E_{\mathrm{p}}$=249 MPa. As can be seen in fig. S2 a), the polymer deformation decreases linearly with the transference number and vanishes for $t^{\mathrm{V}}_{\mathrm{Li}}$=1. This is consistent with the finding that concentration polarization does not occur in single-ion conducting electrolytes. While for $t^{\mathrm{V}}_{\mathrm{Li}}$=1 the lithium flux is only induced by the applied electric field, for $t^{\mathrm{V}}_{\mathrm{Li}} \to 0$ the electric field becomes less important and the lithium motion is mainly induced by diffusion due to the resulting concentration gradients. In fig. S2 b), the polymer deformation decreases with the diffusion coefficient $D^{\mathrm{V}}_{\mathrm{Li}}$ and approaches zero. With a larger diffusion coefficient, the same concentration gradient induces a larger diffusion flux than with a smaller diffusion coefficient. Hence, the stationary state during galvanostatic discharge, in which diffusion and migration fluxes are in equilibrium, requires a smaller concentration gradient and therefore also a smaller polymer deformation. In fig. S2 c), the polymer deformation vanishes for solvent volume ratio both close to 0& and to 100&, and exhibits a maximum for EC vol% $\approx$ 56%. This behaviour of the polymer deformation can be more easily understood when looking at the transport and material factors separately, as shown in fig. S3. In fig. S2 d), the influence of the elastic modulus of the polymer on the polymer deformation can be separated into two regimes. In the regime of small modulus $E_{\mathrm{p}}$<10 MPa, the polymer deformation remains nearly constant. Only when reaching the regime of $E_{\mathrm{p}} \leq$10 MPa, the polymer deformation decreases with larger $E_{\mathrm{p}}$. Since the elastic modulus can regarded as the mechanical resistance against deformations, the corresponding contribution to the (Helmholtz) free energy (see eq. (30)) becomes increasing with larger $E_{\mathrm{p}}$. This leads to an increased the driving force and a decreased material factor $\Theta$ in eq. (S68).

Figure S3 shows the results from the analytical formula eq. (S67) for the transport and material factors $\Xi$ and $\Theta$ in a surface plot, where two of the four parameters $t^{\mathrm{V}}_{\mathrm{Li}}$, $D^{\mathrm{V}}_{\mathrm{Li}}$, EC vol% and $E_{\mathrm{p}}$ are varied. In fig. S3 a), the transport factor $\Xi$ is shown, non-dimensionalized by the multiplication with Faraday's constant $F$ and the reference diffusion coefficient $D^{\mathrm{V}}_{\mathrm{Li},0}$=$1.94 \times 10^{-10}\,\mathrm{m^2\,s^{-1}}$. On the $x$- and $y$-axis, the transference number $t^{\mathrm{V}}_{\mathrm{Li}}$ and the lithium diffusion coefficient $D^{\mathrm{V}}_{\mathrm{Li}}$ are shown, repsectively. As can be seen, the transport factor is very small for $t^{\mathrm{V}}_{\mathrm{Li}} \to 1$, regardless the value of the diffusion coefficient $D^{\mathrm{V}}_{\mathrm{Li}}$. For both smaller $t^{\mathrm{V}}_{\mathrm{Li}}$ and $D^{\mathrm{V}}_{\mathrm{Li}}$ the transport factor increases. The material factor is not shown for different $t^{\mathrm{V}}_{\mathrm{Li}}$ and $D^{\mathrm{V}}_{\mathrm{Li}}$, since it does not depend on those and remains constant (as can be seen in eq. (S68)). In fig. S3 b), the non-dimensionalized transport factor is shown for varying solvent volume ratio EC vol% and elastic modulus $E_{\mathrm{p}}$. It can clearly be seen that the transport factor $\Xi$ depends on the solvent volume ratio, but not on the elastic modulus. For small solvent volume ratios EC vol% < 25%, the transport factor changes only slightly, while for larger values EC vol% > 25% it increases drastically. This is due to $J^2$ appearing in the transport factor (*cf.* eq. (S68)). The solvent volume ratio determines the initial amount of polymer stretch $J$, which is larger for larger EC vol%. Hence, the transport factor increases quadratically with the solvent volume ratio. Figure S3 c) depicts the material factor $\Theta$, non-dimensionalized by the reference material factor $\Theta_0$, which is the material factor evaluated for the reference parameters. The material factor again shows a U-shaped behaviour over the range of the

solvent volume ratio EC vol%, as in fig. S2 c). However, the decrease of $\Theta$ for EC vol%$\rightarrow$0% is much smaller than for EC vol%$\rightarrow$100%. This asymmetry is small for small elastic moduli $E_\mathrm{p}$, but becomes much more pronounced for larger $E_\mathrm{p}$. The elastic modulus can be regarded as a resistance against polymer deformations, so the decrease of the material factor with the elastic modulus is due to the mechanical contributions to the (Helmholtz) free energy (see eq. (30)). The decrease of $\Theta$ with higher EC vol% is a combination of two properties. A higher solvent volume ratio leads to a higher initial stretching of the polymer matrix, *i.e.* $J$ is large. This leads to a high mechanical contribution to the free energy, and therefore a large driving force $\tilde{\mathcal{F}}^\mathrm{V}_{\mathrm{TFSI},c_\mathrm{Li}}$ and a small material factor $\Theta$. The other property is the mixing contribution to the (Helmholtz) free energy. For both small and large EC vol%, the mixing contribution to the (Helmholtz) free energy become large and therefore increase the material factor. The combination of fig. S3 b) and c) explains the behaviour of the polymer deformation seen in fig. S2 c). The multiplication with the transport factor $\Xi$, which is small for small EC vol%, makes the U-shape of the material factor more symmetrical, resulting in the behaviour seen in fig. S2 c).

The resulting polymer deformations are shown in the surface plots fig. 7 in the main text and follow the combination of effects as described above for fig. S2.


[1] A. Kovetz, *Electromagnetic Theory* (Oxford University Press Inc., New York, 2000).
[2] F. Kilchert, M. Lorenz, M. Schammer, P. Nürnberg, M. Schönhoff, A. Latz, and B. Horstmann, arXiv (2022), arXiv:2209.05769.
[3] S. R. de Groot and P. Mazur, *Non-Equilibrium Thermodynamics* (Dover Publications, Inc., New York, 1984).
[4] M. Schammer, B. Horstmann, and A. Latz, Journal of the Electrochemical Society **168**, 026511 (2021).
[5] H. G. Steinrück, C. J. Takacs, H. K. Kim, D. G. MacKanic, B. Holladay, C. Cao, S. Narayanan, E. M. Dufresne, Y. Chushkin, B. Ruta, F. Zontone, J. Will, O. Borodin, S. K. Sinha, V. Srinivasan, and M. F. Toney, Energy and Environmental Science **13**, 4312 (2020).
[6] D. M. Pesko, Z. Feng, S. Sawhney, J. Newman, V. Srinivasan, and N. P. Balsara, Journal of The Electrochemical Society **165**, A3186 (2018).
[7] J. Newman and K. E. Thomas-Alyea, *Electrochemical Systems* (John Wiley & Sons, Inc., 2004).
[8] A. Latz and J. Zausch, Beilstein Journal of Nanotechnology **6**, 987 (2015).
[9] A. Y. Jee, H. Lee, Y. Lee, and M. Lee, Chemical Physics **422**, 246 (2013).
[10] E. E. Ushakova, A. V. Sergeev, A. Morzhukhin, F. S. Napolskiy, O. Kristavchuk, A. V. Chertovich, L. V. Yashina, and D. M. Itkis, RSC Advances **10**, 16118 (2020).
[11] J. Lee, M. Rottmayer, and H. Huang, Journal of Composites Science **6**, 1 (2022).
[12] D. Nikolić, K. A. Moffat, V. M. Farrugia, A. E. Kobryn, S. Gusarov, J. H. Wosnick, and A. Kovalenko, Physical Chemistry Chemical Physics **15**, 6128 (2013).
[13] A. Thum, D. Diddens, and A. Heuer, Journal of Physical Chemistry C **125**, 25392 (2021).
[14] H. D. Nguyen, G. T. Kim, J. Shi, E. Paillard, P. Judeinstein, S. Lyonnard, D. Bresser, and C. Iojoiu, Energy and Environmental Science **11**, 3298 (2018).
[15] A. K. Sahu, S. Pitchumani, P. Sridhar, and A. K. Shukla, Bulletin of Materials Science **32**, 285 (2009).
